# Supplementary material for: Simple models for the trapping of charged particles and macromolecules by diffusiophoresis in salt gradients
Source: arXiv:2512.07442 ancillary file (2025-12-08)

# Calculations for "Simple models for the trapping of charged macromolecules and particles by diffusiophoresis along salt gradients" by Sear and Warren

inspired by experiments, by for example [McDermott et al. \(https://pubs.acs.org/doi/10.1021/la303410w\)](https://pubs.acs.org/doi/10.1021/la303410w).

```
In [1]: import numpy as np
import matplotlib.pyplot as plt
```

## Basic salt properties and DP coefficient

```
In [2]: D_Cl=20.3e-10
print('Cl- D_- ',D_Cl,'m2/s')
D_Na=13.3e-10
print('Na+ D_+ ',D_Na,'m2/s')
D_salt=2.0*D_Na*D_Cl/(D_Na+D_Cl)
print('salt diffusion constant ',D_salt)
print('NaCl salt D ',D_salt,'m2/s')
beta_salt=(D_Na-D_Cl)/(D_Na+D_Cl)
print('beta for salt 1 NaCl ',beta_salt)
#
epsilon0=8.8541e-12
epsilon_water=80*epsilon0
kT=1.3806e-23*(273+20)
# assume deionised water is 10 microM
c_ion_deionised_water_muM=10.0
print('conc of ions (plus or minus) of de-ionised water ',c_ion_dei
onised_water_muM,' uM')
c_ion_deionised_water=c_ion_deionised_water_muM*1.0e-6*6.022e26
print('conc of ions (plus or minus) of de-ionised water ',c_ion_dei
onised_water,' /m^3')
e_elec=1.6021766e-19
Debye_length=np.sqrt(epsilon_water*kT/(2.0*c_ion_deionised_water*e
_elec*2))
print('estimated Debye length in de-ionised water ',Debye_length)

Cl- D_-  2.03e-09 m2/s
Na+ D_+  1.33e-09 m2/s
salt diffusion constant  1.6070833333333333e-09
NaCl salt D  1.6070833333333333e-09 m2/s
beta for salt 1 NaCl  -0.2083333333333333
conc of ions (plus or minus) of de-ionised water  10.0 uM
conc of ions (plus or minus) of de-ionised water  6.021999999999999
e+21 /m^3
estimated Debye length in de-ionised water  9.626960538080732e-08
```

plot some example radial speeds

```

In [3]: lambda_X=1.0e-4
print('lambda_X ',round(lambda_X*1.0e6,2),' um - lengthscale for sa
lt source to dominate')

def uDP_calc_spherical(r1):
    uDP1=-Gamma_DP/(r1+r1**2/lambda_X)
    return uDP1

r_inner=1.0e-5
r_outer=1.0e-3

r_array=np.linspace(r_inner,r_outer,2500)
#
Gamma_DP=1.0e-10
uDP1=uDP_calc_spherical(r_array)
stringy=str(int(Gamma_DP*1.0e12))+ "   $\mathrm{\mu}m^2/s$ "
plt.loglog(r_array/1.0e-6, -uDP1*1.0e6, lw=5, label=stringy)

Gamma_DP=1.0e-11
uDP2=uDP_calc_spherical(r_array)
stringy=str(int(Gamma_DP*1.0e12))+ "   $\mathrm{\mu}m^2/s$ "
plt.loglog(r_array/1.0e-6, -uDP2*1.0e6, lw=5, label=stringy)

plt.loglog([lambda_X*1.0e6, lambda_X*1.0e6], [1.0e-6, 10.0], lw=4, ls
='dotted', color='k')
#
rm1=np.geomspace(10,90,10)
um1=9.0*rm1**(-1)
plt.loglog(rm1,um1,ls=':', lw=4, label='$-1$')
#rm2=np.geomspace(110,190,10)
#um2=9.0*rm1**(-2)
#plt.loglog(rm2,um2,ls=':', lw=3, label='$-2$')
#
plt.xlabel('$r$  ( $\mathrm{\mu}m$ )', fontsize=20)
plt.ylabel('$U_{\mathrm{DP}}$  ( $\mathrm{\mu}m/s$ )', fontsize=20)
plt.ylim([1.0e-2, 1.0e1])
plt.xlim([r_inner*1.0e6, r_outer*1.0e6])
plt.legend(fontsize=20, loc='upper right')
plt.xticks(fontsize=20)
plt.yticks(fontsize=20)
plt.tight_layout()
plt.savefig('UDP3D.pdf')
plt.show()

```

lambda\_X 100.0 um - lengthscale for salt source to dominate

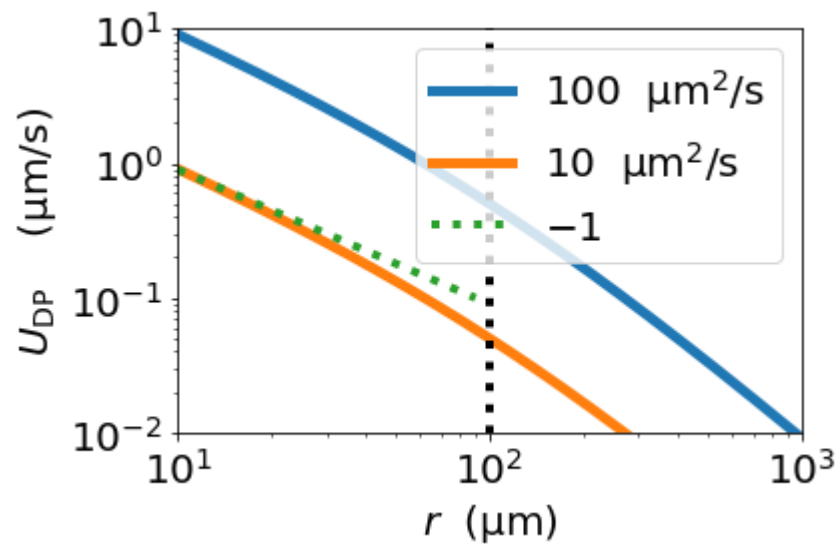

now for plots of steady state concentration near spherical source in large volume

```

In [4]: def csalt_calc_spherical(r1):
        csalt1=lambda_X/r1 + 1.0
        return csalt1

r_inner=1.0e-5
r_outer=1.0e-3
r_array=np.linspace(r_inner,r_outer,25000)
#

# Create a figure and two subplots
fig, (ax1, ax2) = plt.subplots(2, 1, figsize=(6, 8), sharex=True)

#
rho_exponent=-3.0
print('exponent rho ',rho_exponent)
cparticle=(csalt_calc_spherical(r_array)/ \
            csalt_calc_spherical(r_inner))**rho_exponent
ax1.loglog(r_array/1.0e-6,cparticle,lw=5,label='$\\rho=-3$',color
='green')
ax1.loglog(r_array/1.0e-6,(r_array[0]/r_array)**rho_exponent,lw=3,
ls='dashed',color='green')

#
rho_exponent=1.0
print('exponent rho ',rho_exponent)
cparticle=(csalt_calc_spherical(r_array)/ \
            csalt_calc_spherical(r_inner))**rho_exponent
ax1.loglog(r_array/1.0e-6,cparticle,lw=5,label='$\\rho=1$',color
='purple')
ax1.loglog(r_array/1.0e-6,(r_array[0]/r_array)**rho_exponent,lw=3,
ls='dashed',color='purple')

#
rho_exponent=3.0
print('exponent rho ',rho_exponent)
cparticle=(csalt_calc_spherical(r_array)/ \
            csalt_calc_spherical(r_inner))**rho_exponent
ax1.loglog(r_array/1.0e-6,cparticle,lw=5,label='$\\rho=3$',color
='orange')
ax1.loglog(r_array/1.0e-6,(r_array[0]/r_array)**rho_exponent,lw=3,
ls='dashed',color='orange')

#
rho_exponent=10.0
print('exponent rho ',rho_exponent)
#
cparticle=(csalt_calc_spherical(r_array)/ \
            csalt_calc_spherical(r_inner))**rho_exponent
ax1.loglog(r_array/1.0e-6,cparticle,lw=5,label='$\\rho=10$',color
='blue')
ax1.loglog(r_array/1.0e-6,(r_array[0]/r_array)**rho_exponent,lw=3,
ls='dashed',color='blue')

# line at lambda_X
ax1.loglog([lambda_X*1.0e6,lambda_X*1.0e6],[1.0e-6,1.0e6],lw=2,ls
='dotted',color='k',zorder=-9)

```

```

ax1.set_ylabel('$n(r)/n(r=10\mathrm{\mu m})$', fontsize=20)
ax1.set_ylim([1.0e-4, 1.0e3])
ax1.set_xlim([r_inner*1.0e6/1.1, r_outer*1.0e6])
ax1.legend(fontsize=18, loc='upper right')
#ax1.set_xticks(fontsize=20)
#ax1.set_yticks(fontsize=20)
'''

2nd plot
'''

rho_exponent=3.0
print('exponent rho ', rho_exponent)
#lambda_X=10.0e-6
#print('lambda_X', lambda_X)
#cparticle=(csalt_calc_spherical(r_array)/ \
#           csalt_calc_spherical(r_inner))**rho_exponent
#ax2.loglog(r_array/1.0e-6, cparticle, lw=5, label='$\lambda_X=25~\mat
hrm{\mu}m$')
# line at lambda_X
#ax2.loglog([lambda_X*1.0e6, lambda_X*1.0e6], [1.0e-6, 10.0], lw=2, ls
='dotted', color='blue', zorder=-9)
#
lambda_X=20.0e-6
print('lambda_X', lambda_X)
cparticle=(csalt_calc_spherical(r_array)/ \
           csalt_calc_spherical(r_inner))**rho_exponent
ax2.loglog(r_array/1.0e-6, cparticle, lw=5, label='$\lambda_X=20~\mat
hrm{\mu}m$', color='cyan')
ax2.loglog(r_array/1.0e-6, (r_array[0]/r_array)**rho_exponent, lw=4,
ls='dashed', color='cyan')
ax2.loglog([lambda_X*1.0e6, lambda_X*1.0e6], [1.0e-6, 10.0], lw=2, ls
='dotted', color='cyan', zorder=-9)
#
lambda_X=100.0e-6
print('lambda_X', lambda_X)
cparticle=(csalt_calc_spherical(r_array)/ \
           csalt_calc_spherical(r_inner))**rho_exponent
ax2.loglog(r_array/1.0e-6, cparticle, lw=5, label='$\lambda_X=100~\ma
thrm{\mu}m$', color='orange')
ax2.loglog(r_array/1.0e-6, (r_array[0]/r_array)**rho_exponent, lw=2,
ls='dashed', color='orange')
ax2.loglog([lambda_X*1.0e6, lambda_X*1.0e6], [1.0e-6, 1.0e6], lw=2, ls
='dotted', color='orange', zorder=-9)

rho_exponent=-3.0
print('exponent rho ', rho_exponent)
cparticle=(csalt_calc_spherical(r_array)/ \
           csalt_calc_spherical(r_inner))**rho_exponent
#ax2.loglog(r_array/1.0e-6, cparticle, lw=5, label='$\lambda_X=100~\ma
thrm{\mu}m$', color='green')
#ax2.loglog(r_array/1.0e-6, (r_array[0]/r_array)**rho_exponent, lw=3,
ls='dashed', color='green')

ax2.set_ylim([1.0e-4, 1.0e0])
ax2.legend(fontsize=18, loc='upper right')

#plt.xlabel('$r$ ($\mathrm{\mu}m)$', fontsize=20)
ax2.set_xlabel('$r$ ($\mathrm{\mu}m)$', fontsize=20)
ax2.set_ylabel('$n(r)/n(r=10\mathrm{\mu}m)$', fontsize=20)

```

```

# Adjust xtick label size for both subplots
ax1.tick_params(axis='x', labelsz=16)
ax2.tick_params(axis='x', labelsz=16)
ax1.tick_params(axis='y', labelsz=16)
ax2.tick_params(axis='y', labelsz=16)
ax1.text(-0.2, 0.93, '(a)', transform=ax1.transAxes, fontsize=18)
# Add text (b)
ax2.text(-0.2, 0.93, '(b)', transform=ax2.transAxes, fontsize=18)
# Add text (b)

##
plt.tight_layout()
plt.savefig('local3D.pdf')
plt.show()

```

```

exponent rho -3.0
exponent rho 1.0
exponent rho 3.0
exponent rho 10.0
exponent rho 3.0
lambda_X 2e-05
lambda_X 0.0001
exponent rho -3.0

```

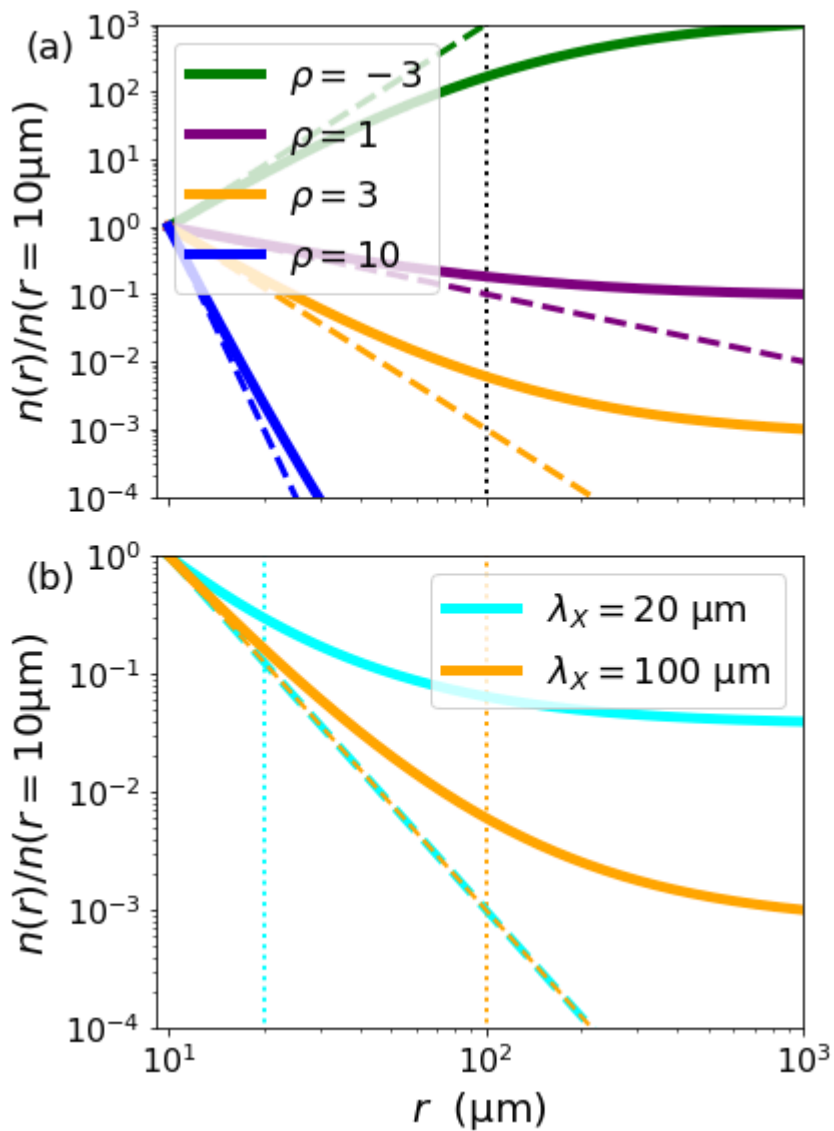

now for 1 D case

```
In [5]: c0=0.1  
        c1=1.0  
        print('c0, c1 ',c0,c1)
```

```
c0, c1  0.1 1.0
```

```

In [6]: L=100.0e-6
print('L length in 1D',L*1.0e6,' um')
#
def U_of_x(x):
    ratio=(c1-c0)/c1
    UDP1D=-(Gamma_DP/L)*ratio/(1.0+ratio*x/L)
    return UDP1D

xplot=np.linspace(0,100.0e-6,200)

Gamma_DP=10.0e-12
print('Gamma',Gamma_DP*1.0e12,' um^2/s')
stringy=str(int(Gamma_DP*1.0e12))+ "  $\mathrm{\mu}$m$^2$/s"
plt.plot(xplot/L,U_of_x(xplot)*1.0e6,lw=5,label=stringy)

Gamma_DP=100.0e-12
print('Gamma',Gamma_DP*1.0e12,' um^2/s')
stringy=str(int(Gamma_DP*1.0e12))+ "  $\mathrm{\mu}$m$^2$/s"
plt.plot(xplot/L,U_of_x(xplot)*1.0e6,lw=5,label=stringy)

plt.xlabel('$x/L$',fontsize=20)
plt.ylabel('$U_{DP}(x)$ ($\mathrm{\mu}$m/s)',fontsize=20)
plt.ylim([-1.0,0.0])
plt.xlim([0,1])
plt.legend(fontsize=20)#,loc='upper right')
plt.xticks(fontsize=20)
plt.yticks(fontsize=20)
plt.tight_layout()
plt.savefig('UDP1D.pdf')
plt.show()

```

L length in 1D 100.0 um  
 Gamma 10.0 um<sup>2</sup>/s  
 Gamma 100.0 um<sup>2</sup>/s

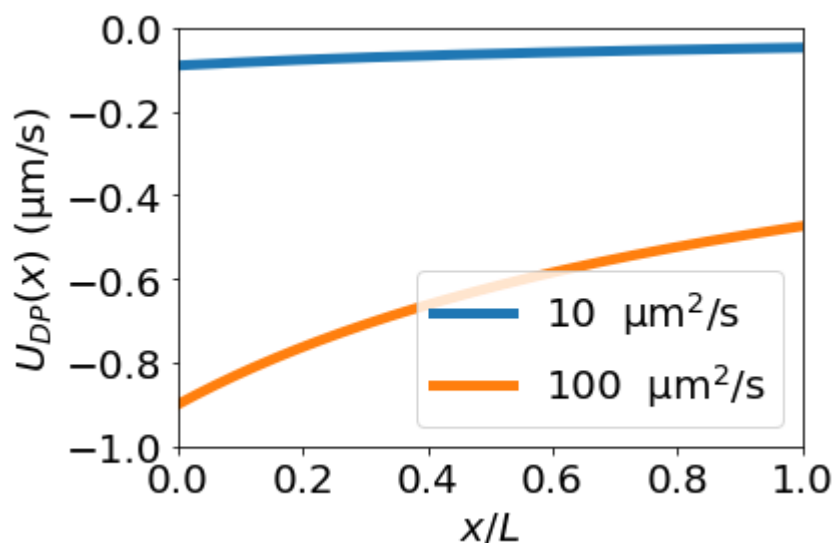



```

In [7]: L=100.0e-6
print('L length in 1D',L*1.0e6,' um')

#
def csalt_of_x(x):
    csalt=c1-(c1-c0)*(x/L)
    return csalt
##

fig, ax1 = plt.subplots(1, 1, figsize=(7, 4.5))

rho1D=2.0
c1Dplot=(csalt_of_x(xplot))**rho1D
ax1.plot(xplot/L,c1Dplot,lw=5,label='$\\rho=2$')

rho1D=20.0
c1Dplot=(csalt_of_x(xplot))**rho1D
ax1.plot(xplot/L,c1Dplot,lw=5,label='$\\rho=20$')

ax1.set_xlabel('$x/L$', fontsize=20)
ax1.set_ylabel('$n(x)/n(x=0)$', fontsize=20)
#plt.ylim([1.0e-3,1.0])

# Adjust xtick label size for both subplots
ax1.tick_params(axis='x', labelsz=16)
ax1.tick_params(axis='y', labelsz=16)

ax1.set_xlim([0,1])
ax1.legend(fontsize=20)#,loc='upper right')
plt.tight_layout()
plt.savefig('local1D.pdf')
plt.show()

```

L length in 1D 100.0 um

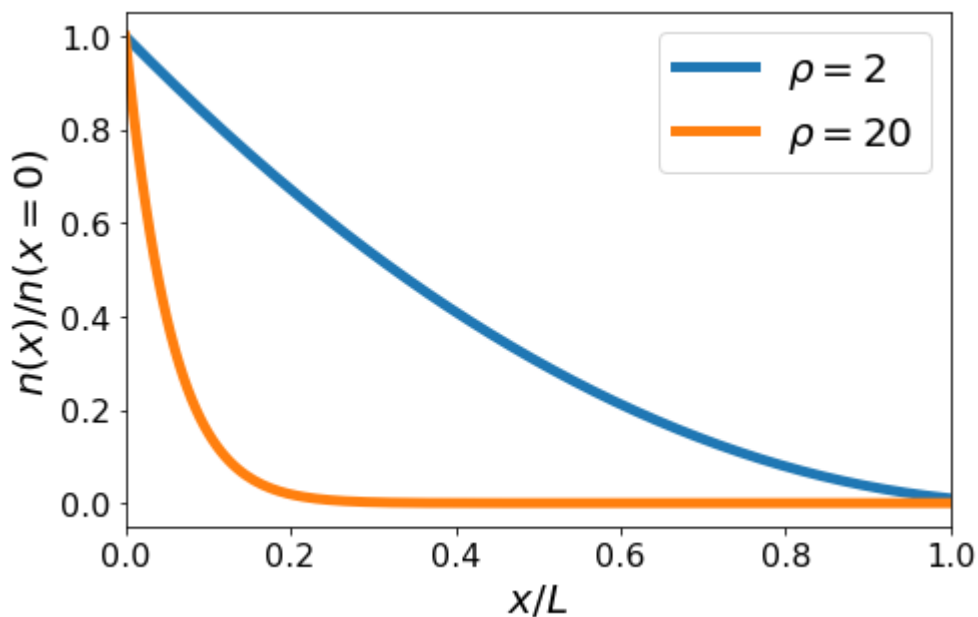

Supplement: Supplementary file 1 [file 2025_static_sourceDPlocalisation.pdf]
